# Supplementary material for: Application-Level Differential Checkpointing for HPC Applications with Dynamic Datasets
Source: arXiv:1906.05038 source file (2019-06-12)
Supplement: Supplementary file 1 [file appendix.tex]

\section{Threshold in Detail}
Equation~\ref{eq:threshold-definition} in section~\ref{sec:threshold}
provides a first approximation for the the benefits that may be
achieved using a \dcp{} mechanism. As we stated earlier, we do not take
into account many things. In this section, we give a more detailed
description of that equation.
\subsection{Saving ($\Delta T_s$)}
Without having \dcp{} enabled, the time for a \cp{} consists primarily
of the time, $\Delta T_0$, that it takes to write $N_t$ blocks of size
$b$. We have:
\begin{equation}
    \Delta T_0 = N_t t_w,
\end{equation}
with $t_w$ being the time that it takes to write one block of size $b$.

Enabling the \dcp{} mechanism leads to the shorter time, $\Delta T_d$,
that it takes to write only $N_d$ blocks. We have:  
\begin{equation}\label{eq:td_bare}
    \Delta T_d = N_d t_w.
\end{equation}
The time difference, or saving, $\Delta T_s$, then is:
\begin{equation}\label{eq:saving_bare}
    \Delta T_s = \Delta T_d - \Delta T_0 = (N_d - N_t) t_w.
\end{equation}
However, we have to take into account, that due to less stress on the
network, the time to write a block will be less for writing $N_d$
instead of $N_t$ blocks. In general we should impose an $N$ dependency
to $t_w$. We can do so by writing equation~\ref{eq:td_bare} differently:
\begin{align}
    \Delta T'_d = N_d t'_w & = N_d (t_w(N_t) - \delta t_w(N_d)) \\
                          & = \Delta T_d - \delta \Delta T_d
\end{align},
where we assume that $\delta \Delta T_d$ is positive. Furthermore, due
to the chunk sizes of dirty data blocks in general not being a multiple
of the block size, we will have in general $N_{d'} = N_d+\delta N_d$
blocks to write. Since the block size of those blocks correspond to a
stochastic quantity, we can not assign one time to all the blocks. We
have rather:
\begin{equation}
    \delta \Delta T_{d'} = \frac{1}{N_{d'}}\sum_i^{N_{d'}} t_w(i),
\end{equation}
Where $\delta \Delta T_{d'}$ clearly is a positive quantity.  For $N_t$,
we have the last block that is smaller then the others and thus related
to a slightly shorter time to write, however, this effect is probably
negligible.   

With this, we may write a corrected term for the saving as:
\begin{mdframed}\begin{align}\label{eq:saving}
    \Delta T'_s & = (N_d - N_t) t_w - N_d \delta t_w + \frac{1}{N_{d'}}\sum_i^{N_{d'}} t_{w,i} \nonumber \\
                & = \Delta T_s - \delta \Delta T_d + \delta \Delta T_{d'}
\end{align}\end{mdframed}
Where the first correction acts in favor and the second not in favor to
the \dcp{} performance.
\subsection{Cost ($\Delta T_c$)}
The cost for the \dcp{} mechanism in FTI, is basically given by the time
that we need to create hashes from the blocks of size $b$. In total we
have to do that $N_t+N_d$ times. Hence, we may write:
\begin{equation}\label{eq:cost_bare}
    \Delta T_c = (N_d + N_t) t_h.
\end{equation}
But similar as for the saving, we have to add a correction to the
cost as well. The term we have to add is in analogy to the second term
we added to the saving:
\begin{equation}
    \delta \Delta T_{c} = \frac{1}{N_{d'}}\sum_i^{N_{d'}} t_h(i),
\end{equation}
Where $N_d'$ is again the additional blocks that will be generated due
to the dirty chunk sizes not being a multiple of the block size $b$.
With this we have the corrected cost:
\begin{align}
    \delta \Delta T'_{c} & = (N_d + N_t) t_h + \frac{1}{N_{d'}}\sum_i^{N_{d'}} t_h(i) \\
                         & = \Delta T_c + \delta \Delta T_{c}
\end{align}
\subsection{Corrected Speedup $\tau'$}
The total time for any \dcp{} update is hence:
\begin{equation}
    \Delta T_{\text{\dcp{}}} = \Delta T_0 + \Delta T'_s + \Delta T'_c
\end{equation}
or the speedup:
\begin{align}
    \Delta T_{\text{su}} & = \Delta T_{\text{\dcp{}}} - \Delta T_0 \nonumber \\
                         & = \Delta T'_s + \Delta T'_c \nonumber \\
                         & = N_t\tau  - \delta \Delta T_d + \delta \Delta T_{d'} + \delta \Delta T_{c} \nonumber \\
                         & = N_t\tau  - N_d \delta t_w + \mathcal{O}(N_{d'})
\end{align}
With this we may write the corrected cost function (compare
equation~\ref{eq:threshold-definition}) as: 
\begin{mdframed}
\begin{equation}
    \tau' = \tau  - n_d \delta t_w(n_d) + \mathcal{O}(n_{d'})
\end{equation}
\end{mdframed}
